# Supplementary material for: Symbolic Constraints in Polyhedral Enclosure and Tetrahedral Decomposition in Genus-0 Polyhedra
Source: arXiv:2508.18222 source file (2026-10-12)
Supplement: Supplementary file 1 [file Supplement.tex]

\pdfoutput=1
\documentclass{article}

\usepackage[english]{babel}
\usepackage[margin=1in]{geometry}
\usepackage{amsmath, amssymb, textcomp}
\usepackage{graphicx}
\usepackage{float}
\usepackage{booktabs}
\usepackage{threeparttable}
\usepackage{tabularx}
\usepackage{array}
\newcolumntype{Y}{>{\centering\arraybackslash}X}
\setlength{\tabcolsep}{4pt}

\usepackage{amsthm}
\theoremstyle{plain}

\theoremstyle{remark}

\theoremstyle{definition}

\usepackage{tikz}
\usepackage{tikz-3dplot}
\usetikzlibrary{arrows.meta,positioning,fit,shadows.blur}
\usepackage{caption}
\usepackage{subcaption}

\newcommand{\tmop}[1]{\ensuremath{\operatorname{#1}}}

\newcommand{\tmstrong}[1]{\textbf{#1}}

\newenvironment{tmindent}{\begin{tmparmod}{1.5em}{0pt}{0pt}}{\end{tmparmod}}
\newenvironment{tmparmod}[3]{
  \begin{list}{}{\setlength{\topsep}{0pt}
  \setlength{\leftmargin}{#1}
  \setlength{\rightmargin}{#2}
  \setlength{\parindent}{#3}
  \setlength{\listparindent}{\parindent}
  \setlength{\itemindent}{\parindent}
  \setlength{\parsep}{\parskip}}
  \item[]
}{\end{list}}

\usepackage[hyphens]{url}
\usepackage[hidelinks,breaklinks=true,bookmarksopen=true,pdfencoding=auto]{hyperref}
\hypersetup{
  pdftitle    = {Supplementary Material: Symbolic Constraints in Polyhedral Enclosure and Tetrahedral Decomposition in Genus-0 Polyhedra},
  pdfauthor   = {Moustapha Itani},
  pdfkeywords = {polyhedral combinatorics, Euler characteristic, triangulations}
}

\begin{document}

\begin{center}
{\Large Supplementary Material for}\\[2pt]
{\Large \emph{Symbolic Constraints in Polyhedral Enclosure and Tetrahedral Decomposition in Genus-0 Polyhedra}}\\[6pt]
Moustapha Itani
\end{center}

\medskip
This document contains appendices and worked examples referenced in the main text.

\appendix

\section{Empirical Worked Examples ($V=4$--$7$)}
\label{supp:empirical}

All results in this appendix are empirical examples obtained by manual
construction. No general existence or completeness claim is made.

\begin{itemize}
  \item $N$: total surface angle units ($180^{\circ}$ each)
  \item $S$: external triangulation segments
  \item $F$: faces; $E$: edges
\item Face counts: $F_k$ denotes the number of $k$-gonal faces
      ($F_3$ triangles, $F_4$ quadrilaterals, $F_5$ pentagons, $F_6$ hexagons)
\item Vertex valencies: $V_k$ denotes the number of vertices of degree $k$
      ($V_3$ through $V_6$)
  \item $T$: tetrahedra; $N_i$: internal gluing triangles; $S_i$: internal triangulation segments
\end{itemize}

\begin{table}[H]
\centering
\caption{Empirical worked configurations for polyhedra with $V=4$ to $V=7$.
Each row represents a manually constructed example. The final two columns
verify Euler's characteristic and the internal consistency relation
$T - N_i + S_i = 1$.}
\label{tab:appendix_empirical_V4to7}
\setlength{\tabcolsep}{5pt}
\renewcommand{\arraystretch}{0.85}
\begin{tabular}{
  c c
  c c c
  c c c c
  c c c c
  c c c
  c c
}
\toprule
$V$ & $N$ &
$S$ & $F$ & $E$ &
$F_3$ & $F_4$ & $F_5$ & $F_6$ &
$V_3$ & $V_4$ & $V_5$ & $V_6$ &
$T$ & $N_i$ & $S_i$ &
$V{-}E{+}F$ & $T{-}N_i{+}S_i$ \\
\midrule
4 & 4 &
0 & 4 & 6 &
4 & -- & -- & -- &
4 & -- & -- & -- &
1 & 0 & 0 &
2 & 1 \\
\midrule
5 & 6 &
0 & 6 & 9 &
6 & 0 & -- & -- &
2 & 3 & -- & -- &
2 & 1 & 0 &
2 & 1 \\
  &   &
1 & 5 & 8 &
4 & 1 & -- & -- &
4 & 1 & -- & -- &
2 & 1 & 0 &
2 & 1 \\
\midrule
6 & 8 &
0 & 8 & 12 &
8 & 0 & 0 & -- &
2 & 2 & 2 & -- &
3 & 2 & 0 &
2 & 1 \\
  &   &
0 & 8 & 12 &
8 & 0 & 0 & -- &
0 & 6 & 0 & -- &
4 & 4 & 1 &
2 & 1 \\
  &   &
1 & 7 & 11 &
6 & 1 & 0 & -- &
2 & 4 & 0 & -- &
3 & 2 & 0 &
2 & 1 \\
  &   &
1 & 7 & 11 &
6 & 1 & 0 & -- &
3 & 2 & 1 & -- &
3 & 2 & 0 &
2 & 1 \\
  &   &
2 & 6 & 10 &
4 & 2 & 0 & -- &
4 & 2 & 0 & -- &
3 & 2 & 0 &
2 & 1 \\
  &   &
2 & 6 & 10 &
5 & 0 & 1 & -- &
5 & 0 & 1 & -- &
3 & 2 & 0 &
2 & 1 \\
  &   &
3 & 5 & 9 &
2 & 3 & 0 & -- &
6 & 0 & 0 & -- &
3 & 2 & 0 &
2 & 1 \\
\midrule
7 & 10 &
0 & 10 & 15 &
10 & 0 & 0 & 0 &
2 & 3 & 0 & 2 &
4 & 3 & 0 &
2 & 1 \\
  &    &
0 & 10 & 15 &
10 & 0 & 0 & 0 &
2 & 2 & 2 & 1 &
4 & 3 & 0 &
2 & 1 \\
  &    &
0 & 10 & 15 &
10 & 0 & 0 & 0 &
1 & 3 & 3 & 0 &
5 & 5 & 1 &
2 & 1 \\
  &    &
0 & 10 & 15 &
10 & 0 & 0 & 0 &
0 & 5 & 2 & 0 &
6 & 7 & 2 &
2 & 1 \\
  &    &
1 & 9 & 14 &
8 & 1 & 0 & 0 &
3 & 2 & 1 & 1 &
4 & 3 & 0 &
2 & 1 \\
  &    &
1 & 9 & 14 &
8 & 1 & 0 & 0 &
3 & 1 & 3 & 0 &
4 & 3 & 0 &
2 & 1 \\
  &    &
1 & 9 & 14 &
8 & 1 & 0 & 0 &
2 & 3 & 2 & 0 &
4 & 3 & 0 &
2 & 1 \\
  &    &
1 & 9 & 14 &
8 & 1 & 0 & 0 &
1 & 5 & 1 & 0 &
5 & 5 & 1 &
2 & 1 \\
  &    &
2 & 8 & 13 &
7 & 0 & 1 & 0 &
3 & 3 & 1 & 0 &
4 & 3 & 0 &
2 & 1 \\
  &    &
2 & 8 & 13 &
6 & 2 & 0 & 0 &
3 & 3 & 1 & 0 &
4 & 3 & 0 &
2 & 1 \\
  &    &
3 & 7 & 12 &
6 & 0 & 0 & 1 &
6 & 0 & 0 & 1 &
4 & 3 & 0 &
2 & 1 \\
  &    &
3 & 7 & 12 &
5 & 1 & 1 & 0 &
4 & 3 & 0 & 0 &
4 & 3 & 0 &
2 & 1 \\
  &    &
3 & 7 & 12 &
4 & 3 & 0 & 0 &
4 & 3 & 0 & 0 &
4 & 3 & 0 &
2 & 1 \\
  &    &
4 & 6 & 11 &
3 & 2 & 1 & 0 &
6 & 1 & 0 & 0 &
4 & 3 & 0 &
2 & 1 \\

\bottomrule
\end{tabular}
\end{table}

No claim is made that the listed configurations exhaust all admissible cases
for the given vertex counts.

\section{Topological Comparison of Tetrahedralization Strategies and Breakdown of the Proposed Identity with Internal Steiner Points}
\label{supp:strategies}

To evaluate how different tetrahedralization strategies affect the internal structure of a cube,
I analyze key topological quantities including the number of tetrahedra \(T\),
internal gluing triangle faces \(N_i\), and internal triangulation segments \(S_i\). The proposed identity
\[
T - N_i + S_i = 1
\]
is observed to hold consistently across minimal and marching tetrahedra configurations,
provided no internal vertices are added. However, once an internal Steiner point is introduced,
particularly when it is treated as an internal vertex connected to new edges or faces,
this relation fails. The following table presents a comparative breakdown of several configurations,
highlighting how modeling assumptions (e.g., counting internal segments as edges or new pyramid faces as external) affect topological consistency.
This analysis reinforces the significance of preserving external-only structure in minimal decompositions
and offers a reference for evaluating topological soundness in more complex triangulations.

\begin{table}[H]
\centering
\caption{Topological comparison of tetrahedralization strategies for a cube.
The identity $T - N_i + S_i = 1$ holds for decompositions without internal
vertices, but fails once an internal Steiner point is introduced under various
counting conventions.}
\label{tab:appendix_steiner_comparison}
\setlength{\tabcolsep}{6pt}
\renewcommand{\arraystretch}{0.9}
\begin{tabular}{lcccccccccc}
\toprule
Configuration
& $V$ & $E$ & $F$
& $T$ & $N_i$ & $S_i$
& $E{-}F$
& $2T{-}N_i$
& $V{-}E{+}F$
& $T{-}N_i{+}S_i$ \\
\midrule
Minimal
& 8 & 12 & 6
& 5 & 4 & 0
& 6 & 6 & 2 & 1 \\
Marching tetrahedralization
& 8 & 12 & 6
& 6 & 6 & 1
& 6 & 6 & 2 & 1 \\
Steiner not counted as vertex
& 8 & 12 & 6
& 12 & 18 & 0
& 6 & 6 & 2 & $-6$ \\
Steiner counted as vertex
& 9 & 12 & 6
& 12 & 18 & 0
& 6 & 6 & 3 & $-6$ \\
Steiner counted + edges
& 9 & 20 & 6
& 12 & 18 & 0
& 14 & 6 & $-5$ & $-6$ \\
Steiner counted + edges + faces
& 9 & 20 & 18
& 12 & 6 & 0
& 2 & 18 & 7 & 6 \\
\bottomrule
\end{tabular}
\end{table}

This comparison demonstrates that the proposed identity is robust when internal structure arises solely from external constraints.
In the minimal 5-tetrahedra decomposition, the identity holds exactly with no added internal triangulation segments.
In the marching tetrahedralization strategy, although the identity still holds, the cube is bisected into two hexahedra by introducing an internal quadrilateral face.
This increases internal complexity: one additional tetrahedron is required (\(T\) increases by 1), along with two new internal gluing triangles (\(N_i\))
and one internal triangulation segment (\(S_i\)). Nonetheless, the identity is preserved due to the balance between these added quantities.
However, once a Steiner point is introduced inside the volume and treated as a vertex connected by new internal edges or faces, the identity fails.
This breakdown reflects a fundamental shift in the topological model: the internal structure is no longer a consequence of surface triangulation alone,
but instead includes additional volumetric elements. These results emphasize the importance of distinguishing between surface-conforming decompositions
and those requiring internal augmentation when analyzing or designing tetrahedral meshes.

 \medskip
\noindent\textbf{Interpretation.}
In the rows where interior faces/edges are counted together with boundary faces/edges,
the quantity $V-E+F$ is no longer the Euler characteristic of a $2$--cell embedding of a closed surface.
Rather, it is a mixed bookkeeping statistic for a $3$--dimensional cell complex.
Accordingly, values such as $9-20+18=7$ do \emph{not} indicate a failure of Euler's formula;
they indicate that the counted $(V,E,F)$ do not describe the boundary sphere alone.
For the boundary $2$--complex (faces only on $\partial$), one still has $V-E+F=2$.
Now, compare with Appendix C for a case where invariance is preserved under surface-Steiner points.

\section{Invariance of the Proposed Identity for Polyhedra with Surface-Embedded Edge Steiner Points}
\label{supp:invariance}

To illustrate the invariance of the identity $T - N_i + S_i = 1$ under different
tetrahedral decompositions, including those involving Steiner points, consider
a single tetrahedron with one Steiner point placed on each of three edges,
each edge chosen such that the three Steiner points lie \ on the same face.

{\tmstrong{Decomposition A (Plane Cut Through Three Steiner Points):}}\\
Consider the plane passing through the three Steiner points. This plane
divides the tetrahedron into two polyhedral regions:
\begin{itemize}
  \item One region is a tetrahedron.
  
  \item The other is a five-faced polyhedron bounded by three quadrilateral
  faces and two triangular faces, with six vertices in total.
\end{itemize}
This five-faced polyhedron can be further decomposed into {\tmstrong{three
tetrahedra}}, yielding a total of {\tmstrong{four tetrahedra}}. The tetrahedra
are glued pairwise along {\tmstrong{three internal triangular faces}}, and the
only Steiner points used are the original three placed on the edges.

Thus, the identity is satisfied:
\[ T = 4, N_i = 3, S_i = 0 \Rightarrow T - N_i + S_i = 4 - 3 + 0 = 1 \]

{\tmstrong{Decomposition B (Edge-Based Slicing Through Steiner Points):}}\\
Alternatively, one can sequentially slice the tetrahedron through one Steiner
point at a time, joining each to the two original vertices that define its
edge, and to one of the remaining original vertices, forming tetrahedra that
share triangular faces. This approach also produces {\tmstrong{four
tetrahedra}}, glued across the same number of internal triangular interfaces
({\tmstrong{three}}), and using the same {\tmstrong{three Steiner points}}.

Again, the identity holds:
\[ T - N_i + S_i = 4 - 3 + 0 = 1 \]
This example shows that {\tmstrong{despite the different topology of the
intermediate polyhedral shapes}}, the identity is preserved, emphasizing its
{\tmstrong{combinatorial invariance}} across Steiner-supported decompositions.

\section{Worked Examples Demonstrating the Combinatorial Method
for Testing 3D Polygonal Enclosure and Feasibility}
\label{supp:examples}

This appendix presents worked examples that demonstrate the combinatorial
method. It includes three examples that are combinatorially and geometrically
valid, one example that is too flat to enclose, and an example of a likely
false positive, a case where the set of polygons is determined symbolically
valid but likely unrealizable.

\subsection*{Worked Example: Four Triangles and One Quadrilateral (Square
Pyramid)}

\begin{itemize}
  \item Step 1: Polygons: 1 square ($P_4 = 1$), 4 triangles ($P_3 = 4$)
  \item Step 2: $N = 6$
  \item Step 3: $V = \frac{6}{2} + 2 = 5$
  \item Step 4: $S = 1$
  \item Step 5: $F = 5$
  \item Step 6: $E = 3 \cdot (5 - 2) - 1 = 8$
  \item Step 7: Euler check: $5 - 8 + 5 = 2$
  \item Step 8: $S_{\mathrm{ub}} = \frac{3}{2} \cdot 5 - \tfrac{13}{2} = 2$;
  $S_{\mathrm{difference}} = 1$ (passes flatness test)
\end{itemize}

\subsection*{Worked Example: Six Squares (The Cube)}

\begin{itemize}
  \item Step 1: Polygons: 6 squares or quadrilaterals ($P_4 = 6$)
  \item Step 2: $N = (4 - 2) \cdot 6 = 12$
  \item Step 3: $V = \frac{12}{2} + 2 = 8$
  \item Step 4: $S = (4 - 3) \cdot 6 = 6$
  \item Step 5: $F = 6$
  \item Step 6: $E = 3 \cdot (8 - 2) - 6 = 12$
  \item Step 7: Euler check: $8 - 12 + 6 = 2$
  \item Step 8: $S_{\mathrm{ub}} = \frac{3}{2} \cdot 8 - 6 = 6$;
  $S_{\mathrm{difference}} = 0$ (passes flatness test)
\end{itemize}

\subsection*{Worked Example: 12 Pentagons (The Dodecahedron)}

\begin{itemize}
  \item Step 1: Polygons: 12 pentagons ($P_5 = 12$)
  \item Step 2: $N = (5 - 2) \cdot 12 = 36$
  \item Step 3: $V = \frac{36}{2} + 2 = 20$
  \item Step 4: $S = (5 - 3) \cdot 12 = 24$
  \item Step 5: $F = 12$
  \item Step 6: $E = 3 \cdot (20 - 2) - 24 = 30$
  \item Step 7: Euler check: $20 - 30 + 12 = 2$
  \item Step 8: $S_{\mathrm{ub}} = \frac{3}{2} \cdot 20 - 6 = 24$;
  $S_{\mathrm{difference}} = 0$ (passes flatness test)
\end{itemize}

\subsection*{Worked Example: 36 Hexagons}

\begin{itemize}
  \item Step 1: Polygons: 36 hexagons ($P_6 = 36$)
  \item Step 2: $N = 144$
  \item Step 3: $V = \frac{144}{2} + 2 = 74$
  \item Step 4: $S = 108$
  \item Step 5: $F = 36$
  \item Step 6: $E = 3 \cdot (74 - 2) - 108 = 108$
  \item Step 7: Euler check: $74 - 108 + 36 = 2$
  \item Step 8: $S_{\mathrm{ub}} = \frac{3}{2} \cdot 74 - 6 = 105$;
  $S_{\mathrm{difference}} = -3$ (fails flatness test)
\end{itemize}
\begin{tmindent}
  \textbf{Conclusion: }A set of 36 hexagons cannot produce an enclosed
  polyhedron.
\end{tmindent}

\subsection*{Worked Example: Two Hexagons and Four Triangles (False Positive)}

\begin{itemize}
  \item \textbf{Step 1:} Polygons: 2 hexagons ($P_6 = 2$), 4 triangles ($P_3 = 4$)
  \item \textbf{Step 2:} $N = (6 - 2) \cdot 2 + (3 - 2) \cdot 4 = 8 + 4 = 12$
  \item \textbf{Step 3:} $V = \frac{12}{2} + 2 = 8$
  \item \textbf{Step 4:} $S = (6 - 3) \cdot 2 + (3 - 3) \cdot 4 = 6 + 0 = 6$
  \item \textbf{Step 5:} $F = 6$
  \item \textbf{Step 6:} $E = 3 \cdot (8 - 2) - 6 = 12$
  \item \textbf{Step 7:} Euler check: $V - E + F = 8 - 12 + 6 = 2$ (passes)
  \item \textbf{Step 8:} $S_{\mathrm{ub}} = \frac{3}{2} \cdot 8 - 6 = 6$,
  $S_{\mathrm{difference}} = 0$ (passes flatness)
\end{itemize}
\begin{tmindent}
  \textbf{Conclusion:} This configuration passes all combinatorial checks:
  Euler's formula holds, edge and face counts are consistent, the
  triangulation segment count meets the flatness threshold, and a minimal
  internal tetrahedral decomposition is arithmetically feasible. However, no
  known convex or non-convex polyhedron with exactly two hexagons and four
  triangles exists in the literature. The structure cannot be embedded in
  $\mathbb{R}^3$ as a genus-zero surface with non-self-intersecting faces.
  This mismatch illustrates the boundary between symbolic sufficiency and
  geometric feasibility. While the framework successfully captures algebraic
  consistency, it cannot, by design, account for spatial constraints such as
  embeddability or convex closure. This example thus serves as a clear case
  where realizability remains unresolved. No known convex or non-convex realization exists.

  When substituting two of the triangles with one quadrilateral, keeping the
  total face count at six, the resulting configuration becomes {\em too
  flat} to enclose. This failure highlights how even minimal changes in
  polygonal composition can push a structure past the limits of combinatorial
  enclosure. Such sensitivity underscores the \textbf{brittleness} of symbolic
  tetrahedral enclosure near flatness thresholds. The substitution of two
  triangles with a quadrilateral may therefore serve as a practical
  diagnostic for testing the \textbf{combinatorial resilience} of enclosure
  candidates. Identifying and interpreting such tipping points offers a
  pathway for refining this framework and integrating embeddability heuristics
  in future work.
\end{tmindent}

\section{Numerical values of $\mathrm{Combinations}_{\mathrm{lb}}(V)$}
\label{supp:combinations}

\begin{table}[H]
\centering
\caption{Lower-bound estimates of the number of admissible external--internal
macro-configuration pairs, $\mathrm{Combinations}_{\mathrm{lb}}(V)$, as a function of vertex count $V$.}
\label{tab:V4to20_counts}
\setlength{\tabcolsep}{7pt}
\renewcommand{\arraystretch}{0.9}
\begin{tabular}{cc}
\toprule
$V$ & Estimated total configuration sets \\
\midrule
4  & 1  \\
5  & 2  \\
6  & 5  \\
7  & 8  \\
8  & 13 \\
9  & 18 \\
10 & 25 \\
11 & 32 \\
12 & 41 \\
13 & 50 \\
14 & 61 \\
15 & 72 \\
16 & 85 \\
17 & 98 \\
18 & 113\\
19 & 128\\
20 & 145\\
\bottomrule
\end{tabular}
\end{table}

\begin{figure}[H]
  \centering
  \includegraphics[width=11.2917650531287cm,height=6.27320280729372cm]{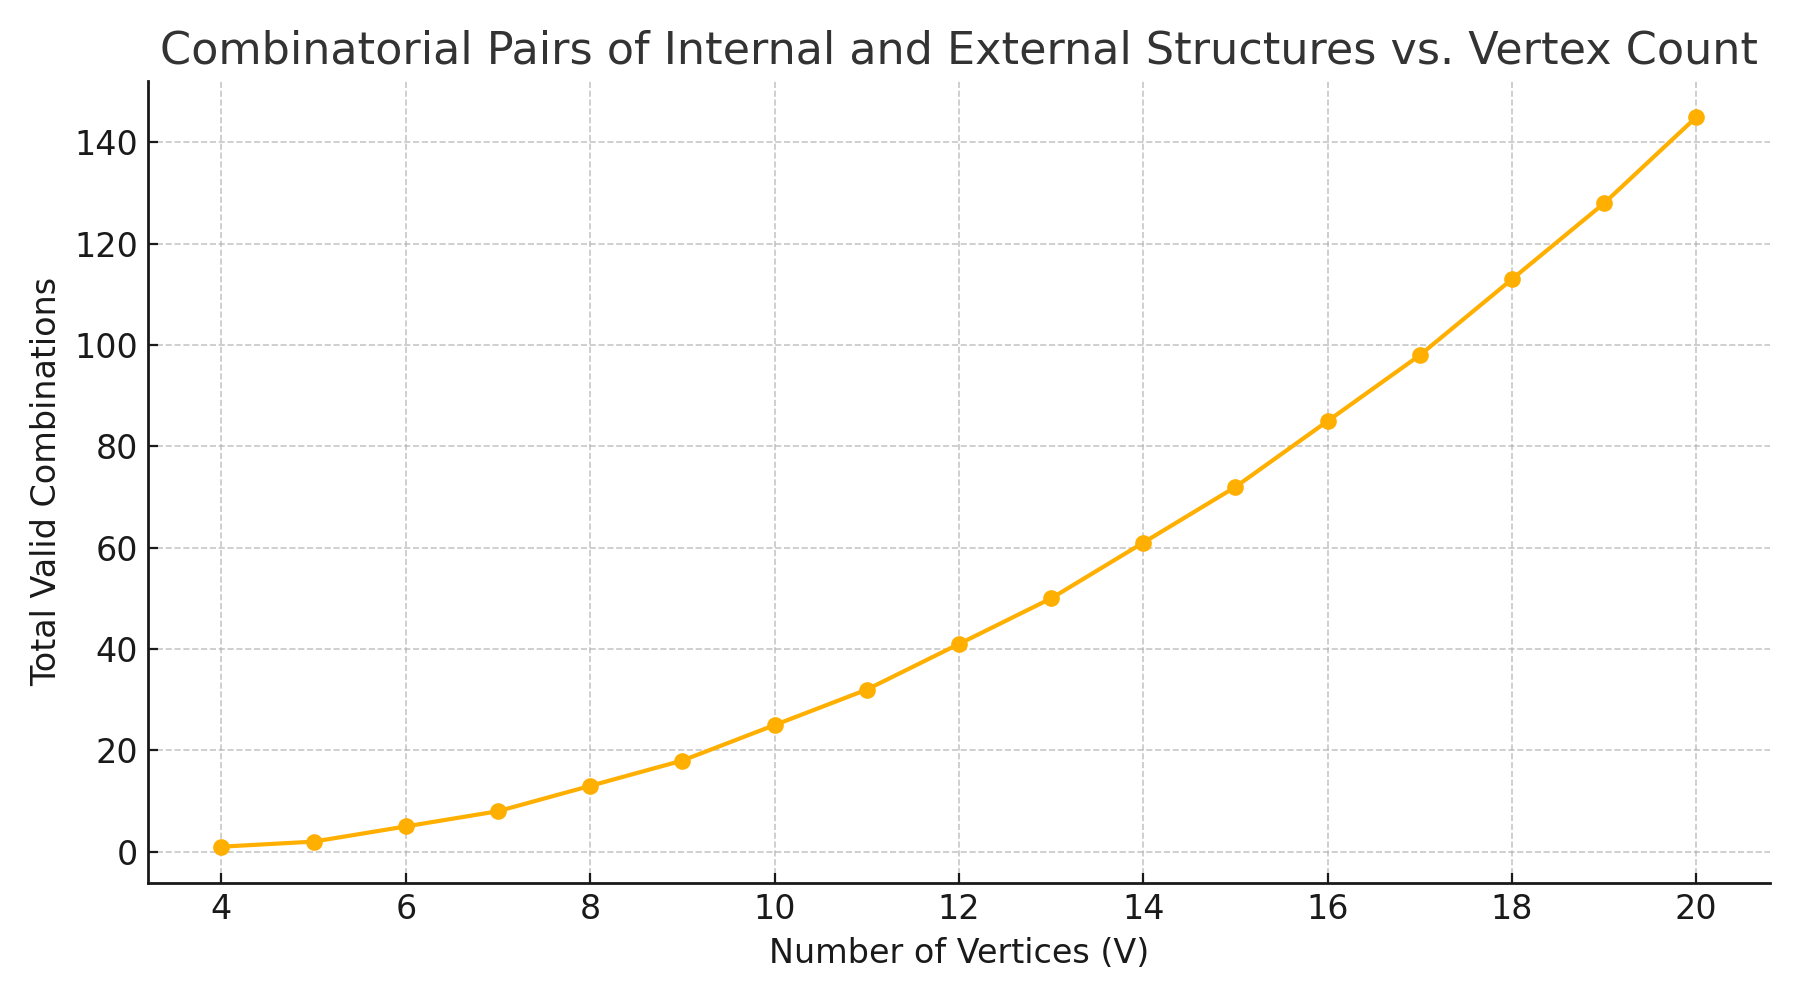}
  \caption{Combinatorial sum of internal and external structure groupings as a function of vertex count.}
\end{figure}

\section{Combinatorial Identities and Bounds}
\label{supp:identities}

This appendix records (i) \emph{proved} external and topological identities used in the main text, and (ii) the \emph{empirical/heuristic} identities and bounds collected from worked decompositions. All variables are symbolic and coordinate-free. Genus~$0$ and normal-form assumptions apply where stated. All linear ``max'' values quoted below are valid within the SALT+MIE class. Non--SALT triangulations can exceed these bounds.

\subsection{Proved External Identities and Bounds}

Exact external formulas for genus-0 polyhedra in normal form:
\begin{align}
  E &= 3V - 6 - S \tag{E.1}\label{appE:E1}\\
  F &= 2V - 4 - S \tag{E.2}\label{appE:E2}
\end{align}
where 
\[
S \;=\; \sum_{f} (\tmop{deg} f - 3) \quad\text{(flatness, total deviation from triangulation).}
\]

From the vertex degree constraint $\tmop{deg}(v) \ge 3$, one obtains the sharp bounds:

\medskip
\noindent
Even $V$:
\begin{align}
  0 &\le S \le \frac{3V}{2}-6, \tag{E.3a}\label{appE:E3a}\\
  \frac{3V}{2} &\le E \le 3V-6, \tag{E.4aE}\\
  \frac{V}{2}+2 &\le F \le 2V-4. \tag{E.4aF}
\end{align}

\noindent
Odd $V$:
\begin{align}
0 &\le S \le \tfrac{3V}{2} - \tfrac{13}{2} \tag{E.3b}\label{appE:E3b}\\
\tfrac{3V+1}{2} &\le E \le 3V - 6 \tag{E.4bE}\label{appE:E4bE}\\
\tfrac{V}{2} + \tfrac{5}{2} &\le F \le 2V - 4 \tag{E.4bF}\label{appE:E4bF}
\end{align}

\medskip
\noindent\textbf{Extremal Values Summary (genus-0, normal form)}  
\begin{center}
\begin{tabular}{c|c|c|c|c|c}
$V$ parity & $S_{\mathrm{ub}}$ & $E_{\mathrm{lb}}$ & $E_{\mathrm{ub}}$ & $F_{\mathrm{lb}}$ & $F_{\mathrm{ub}}$ \\
\hline
Even $V$ & $\dfrac{3V}{2} - 6$ & $\dfrac{3V}{2}$ & $3V - 6$ & $\dfrac{V}{2} + 2$ & $2V - 4$ \\
Odd $V$ & $\dfrac{3V}{2} - \tfrac{13}{2}$ & $\dfrac{3V+1}{2}$ & $3V - 6$ & $\dfrac{V}{2} + \tfrac{5}{2}$ & $2V - 4$ \\
\end{tabular}
\end{center}

\medskip
Angle-unit bookkeeping (fully triangulated boundary):
\begin{align}
  F_{\triangle} &= F + S \;=\; 2V - 4 \tag{E.5}\label{appE:E5}\\
  F_{\triangle} &= 4T - 2N_i \tag{E.6}\label{appE:E6}
\end{align}
(Equation~\eqref{appE:E6} counts triangle units: each tetrahedron contributes $4$, each internal gluing triangle cancels $2$.)

\subsection{Proved Topological Identity for 3D Complexes}

For any tetrahedralization of a $3$--ball (genus--0 volume) with $V_i$ interior vertices and $E_i$ interior edges,
\begin{align}
  T - N_i + E_i - V_i &= 1 \tag{E.7}\label{appE:E7}
\end{align}
(Prop.~\ref{prop:exact-euler}). In particular, when $V_i=0$ (normal form, no interior vertices),
\begin{align}
  T - N_i + E_i &= 1. \tag{E.8}\label{appE:E8}
\end{align}

\subsection{Bridge to the Heuristic Extended Euler Form}

A heuristic identity used in the text is
\begin{align}
  V - E + F &= 2\,(T - N_i + S_i) \tag{E.9h}\label{appE:E9h}
\end{align}
and the SALT ladder case asserts
\begin{align}
  T - N_i + S_i &= 1. \tag{E.10h}\label{appE:E10h}
\end{align}

\noindent\textbf{Convention (SALT+MIE).}
In the SALT+MIE setting we identify $S_i$ with the interior--edge count $E_i$;
outside SALT+MIE, $S_i$ denotes the number of interior triangulation segments
used in the chosen refinement and need not coincide with $E_i$.

\medskip
These coincide with \eqref{appE:E7}--\eqref{appE:E8} whenever $V_i=0$ and
$S_i = E_i$ (as in SALT+MIE constructions).

\bigskip

\subsection{Core Equations (proved unless marked heuristic)}

\begin{align}
  \text{(E.9h)} \quad & V - E + F = 2 (T - N_i + S_i) \quad\text{(heuristic)}\\
  \text{(E.10h)} \quad & T - N_i + S_i = 1 \quad\text{(SALT ladder case)}\\
  \text{(E.11r)} \quad & N_i = 2T - V + 2 \quad\text{(exact in normal form; no interior vertices)}\\
  \text{(E.12r)} \quad & E - F = 2T - N_i \quad\text{(from \eqref{appE:E1}--\eqref{appE:E2} + Euler)}
\end{align}

\subsection{Restricted SALT+MIE ranges (heuristic / construction--based)}

\begin{align}
  \text{(E.13r)} \quad & T_{\min} = V - 3 \\
  \text{(E.14r)} \quad & T_{\max} = 2 (V - 4) \\
  \text{(E.15r)} \quad & N_{i,\min} = V - 4 \\
  \text{(E.16r)} \quad & N_{i,\max} = 3 (V - 4) - 2 
\end{align}

\subsection{Derived Relationships (algebraic within SALT+MIE)}

The following are algebraic consequences of (E.13r)--(E.16r); they are not independent results.

\begin{align}
  \text{(E.17r)} \quad & T_{\max} = 2 N_{i,\min} \\
  \text{(E.18r)} \quad & N_{i,\max} = \tfrac{3}{2} T_{\max} - 2 \\
  \text{(E.19r)} \quad & N_{i,\max} = 2 N_{i,\min} + (V - 6) \\ 
  \text{(E.20r)} \quad & N_{i,\max} - T_{\max} = N_{i,\min} - 2 \\
  \text{(E.21r)} \quad & N_{i,\max} - T_{\max} = T_{\min} - 3 \\
  \text{(E.22r)} \quad & N_{i,\min} = T_{\min} - 1 \\
  \text{(E.23r)} \quad & 2 N_{i,\max} - 2 T_{\max} = N_{i,\min} + T_{\min} - 5 
\end{align}

\bigskip
\noindent\textit{Scope note.} 
Equations (E.1)--(E.8) are exact and universal topological identities. 
Equations (E.9h)--(E.23r) hold only heuristically or within the restricted SALT+MIE construction class.

\end{document}
